# Supplementary material for: Diverse Weight Averaging for Out-of-Distribution Generalization
Source: arXiv:2205.09739 source file (2023-01-27)
Supplement: Supplementary file 1 [file 10_app_dwa_of_ma.tex]

\subsection{DWA of MA}

complementarity between our approach and MA
combine checkpoints from same run and differnent runs

% {e0_acc_net: 66.3, e0_acc_netm: 59.3, e0_acc_soup: 66.9, e0_acc_soupswa: 67.2, e0_acc_swa: 67.2, e0_acc_swam: 65.4, gpu: 0, length: 40}
% {e0_acc_net: 66.2, e0_acc_netm: 59.0, e0_acc_soup: 68.0, e0_acc_soupswa: 67.6, e0_acc_swa: 67.2, e0_acc_swam: 65.6, gpu: 0, length: 40}
% {e0_acc_net: 66.0, e0_acc_netm: 60.6, e0_acc_soup: 67.2, e0_acc_soupswa: 66.3, e0_acc_swa: 65.9, e0_acc_swam: 64.5, gpu: 0, length: 40}
% {e0_acc_net: 66.7, e0_acc_netm: 59.6, e0_acc_soup: 68.2, e0_acc_soupswa: 67.5, e0_acc_swa: 66.9, e0_acc_swam: 65.1, gpu: 0, length: 120}

\begin{table}[h]%
    \caption{\textbf{DiWA vs MA} are complementary in OfficeHome domain `Art`.}
    \centering
    \adjustbox{width=0.7\textwidth}{
        \begin{tabular}{lccc}
            \toprule
            \textbf{Algorithm}               & \textbf{Weights selection} & \textbf{$M=20$} & \textbf{$M=60$} \\
            \midrule
            ERM                              & N/A                        & 62.9 $\pm$ 1.3                    \\
            MA                               & Uniform $M=4900$           & 65.0 $\pm$ 0.2                    \\
            \midrule
            DiWA                              & Uniform: $M=20$            & 67.3 $\pm$ 0.2                    \\
            DiWA$^{\dagger}$                  & Uniform: $M=60$            & 67.7
            \midrule
            DiWA of MA                        & Uniform: $M=20\times 4900$ & 66.7 $\pm$ 0.4                    \\
            DiWA$^{\dagger}$ of MA            & Uniform: $M=60\times 4900$ & 67.3                              \\
            \midrule
            DiWA of best and last             & Uniform: $M=20\times 2$    & 67.4 $\pm$ 0.3                    \\
            DiWA$^{\dagger}$ of best and last & Uniform: $M=60\times 2$    & 68.2                              \\
            \bottomrule
        \end{tabular}}
    \label{table:db_home0_dwa_of_ma}%
\end{table}

% {e0_acc_net: 66.4, e0_acc_netm: 59.9, e0_acc_soup: 67.5, e0_acc_soupswa: 66.8, e0_acc_swa: 67.2, e0_acc_swam: 65.1, gpu: 0, length: 20}
% {e0_acc_net: 65.9, e0_acc_netm: 59.5, e0_acc_soup: 67.7, e0_acc_soupswa: 67.4, e0_acc_swa: 67.0, e0_acc_swam: 65.5, gpu: 0, length: 20}
% {e0_acc_net: 66.0, e0_acc_netm: 60.9, e0_acc_soup: 66.9, e0_acc_soupswa: 65.8, e0_acc_swa: 65.6, e0_acc_swam: 64.3, gpu: 0, length: 20}
% {e0_acc_net: 66.5, e0_acc_netm: 60.1, e0_acc_soup: 67.7, e0_acc_soupswa: 67.3, e0_acc_swa: 66.7, e0_acc_swam: 65.0, gpu: 0, length: 60}
